# Supplementary material for: Accurate electronic band gaps of two-dimensional materials from the local modified Becke-Johnson potential
Source: arXiv:2004.07632 source file (2020-04-16)
Supplement: Supplementary file 1 [file supplement.pdf]

# Electronic band gaps of 2D materials by local modified Becke-Johnson potential (Supplementary Material

**Tomáš Rauch**[1], **Miguel A L Marques**[2,3], **Silvana Botti**[1,3]

[1] Institut für Festkörpertheorie und -optik, Friedrich-Schiller-Universität Jena, Max-Wien-Platz 1, 07743 Jena, Germany

[2] Institut für Physik, Martin-Luther-Universität Halle-Wittenberg, 06120 Halle/Saale, Germany

[3] European Theoretical Spectroscopy Facility

E-mail: `tomas.rauch@uni-jena.de`

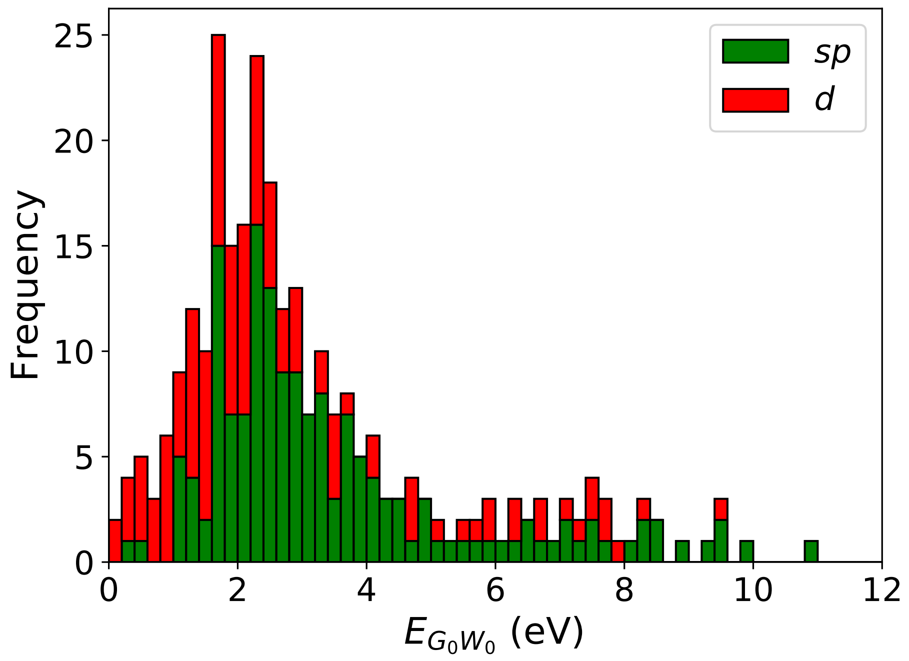


**Figure 1.** Distribution of the $G_0W_0$ band gaps in the C2DB data set [1]. The size of the boxes is 0.2 eV.

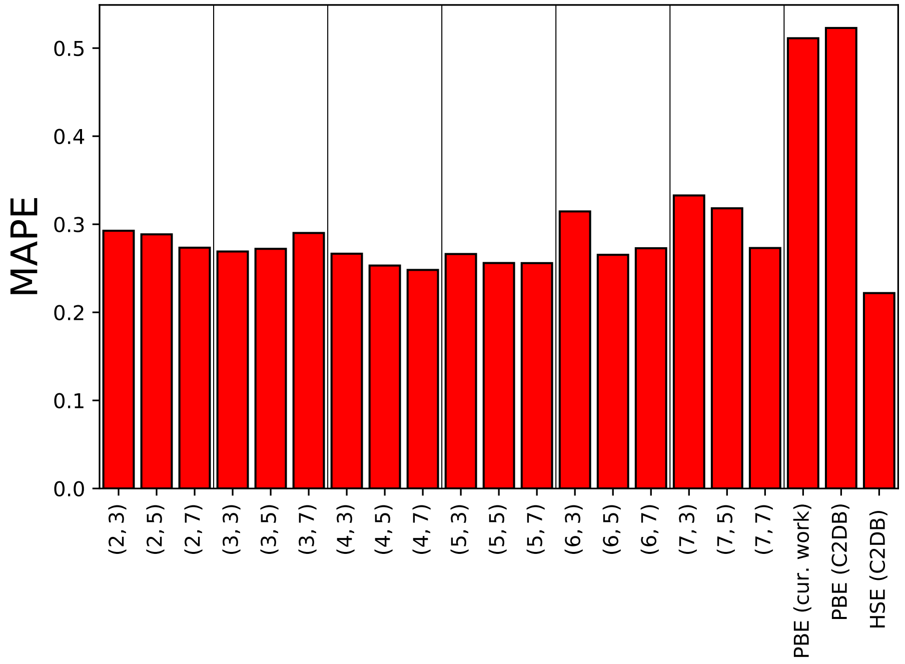


**Figure 2.** Mean absolute percentage error (MAPE) for different values of $(\sigma, r_s^{\mathrm{th}})$ parameters compared with PBE and HSE06 values.

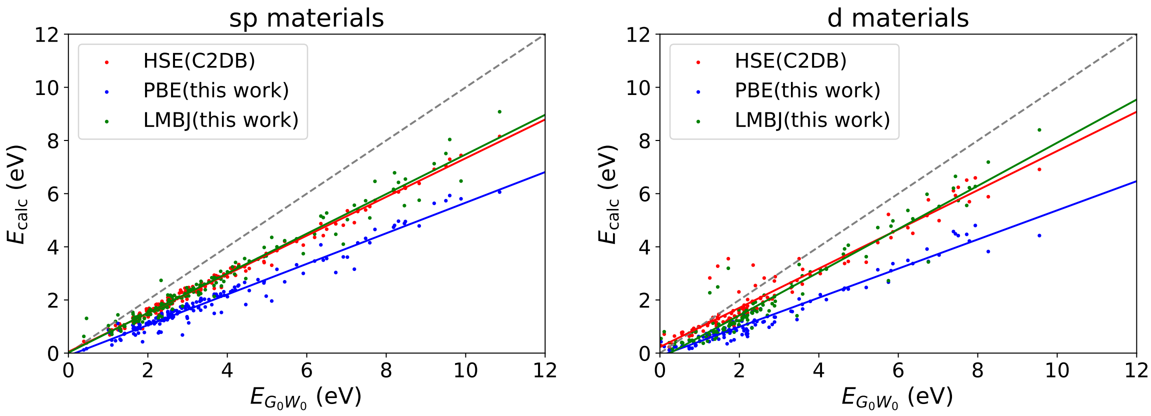


**Figure 3.** Calculated band gaps as a function of $G_0W_0$ (C2DB) band gaps for the data sets "*sp* materials" (left) and "*d* materials" (right). Full lines are linear fits ($y = ax+b$) to the respective data with $a$ and $b$ given in the main text.

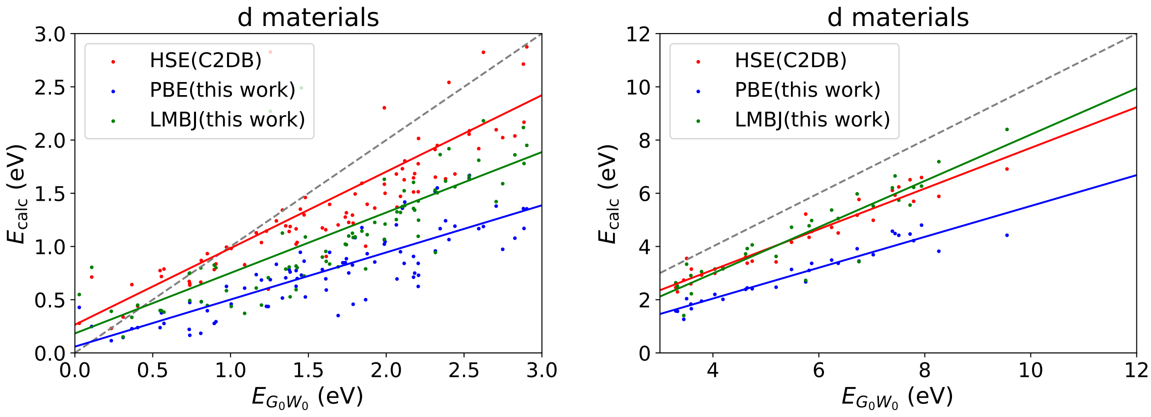


**Figure 4.** Calculated band gaps as a function of $G_0W_0$ (C2DB) band gaps for the data sets "*d* materials with $E_{G_0W_0} \in (0, 3)$ eV" (left) and "*d* materials with $E_{G_0W_0} \in (3, 12)$ eV" (right). Full lines are linear fits ($y = ax + b$) to the respective data with $a$ and $b$ given in the main text.

## References

[1] Haastrup S, Strange M, Pandey M, Deilmann T, Schmidt P S, Hinsche N F, Gjerding M N, Torelli D, Larsen P M, Riis-Jensen A C, Gath J, Jacobsen K W, Mortensen J J, Olsen T and Thygesen K S 2018 *2D Mater.* **5** 042002 URL https://doi.org/10.1088%2F2053-1583%2Faacfc1
